# Supplementary material for: AgentsEval: Clinically Faithful Evaluation of Medical Imaging Reports via Multi-Agent Reasoning
Source: arXiv:2601.16685 source file (2026-01-23)
Supplement: Supplementary file 1 [file X_suppl.tex]

\clearpage
\setcounter{page}{1}
\maketitlesupplementary
\section{Case Studies and Full Reasoning Workflows}

We present detailed case studies illustrating the end-to-end evaluation workflow of AgentsEval.
Each example includes 
(1) the original radiology report, 
(2) multiple model-generated reports, and
(3) the complete intermediate inference chain produced by each agent, including base\_criteria, dynamic\_criteria, gt\_values\_dict, pred\_values\_dict (shown in the figures for A3 rewrite and B3 rewrite), and pred\_score\_details.
These results demonstrate how the multi-agent architecture decomposes evaluation into interpretable steps.

\subsection{Case 1 — Dataset CT-RATE)}

Case 1 compares two rewrite versions (A3, B3) that differ in lexical fluency and subtle clinical phrasing.
Although both appear fluent, AgentsEval uncovers several clinically relevant inconsistencies, including missing modifiers and altered diagnostic certainty.
These findings highlight the need for interpretable clinical evaluation instead of surface-level similarity metrics. All the details are shown in the Figure~\ref{fig:Ex_1}.

\begin{figure*}[t]
    \centering
    \includegraphics[width=\textwidth]{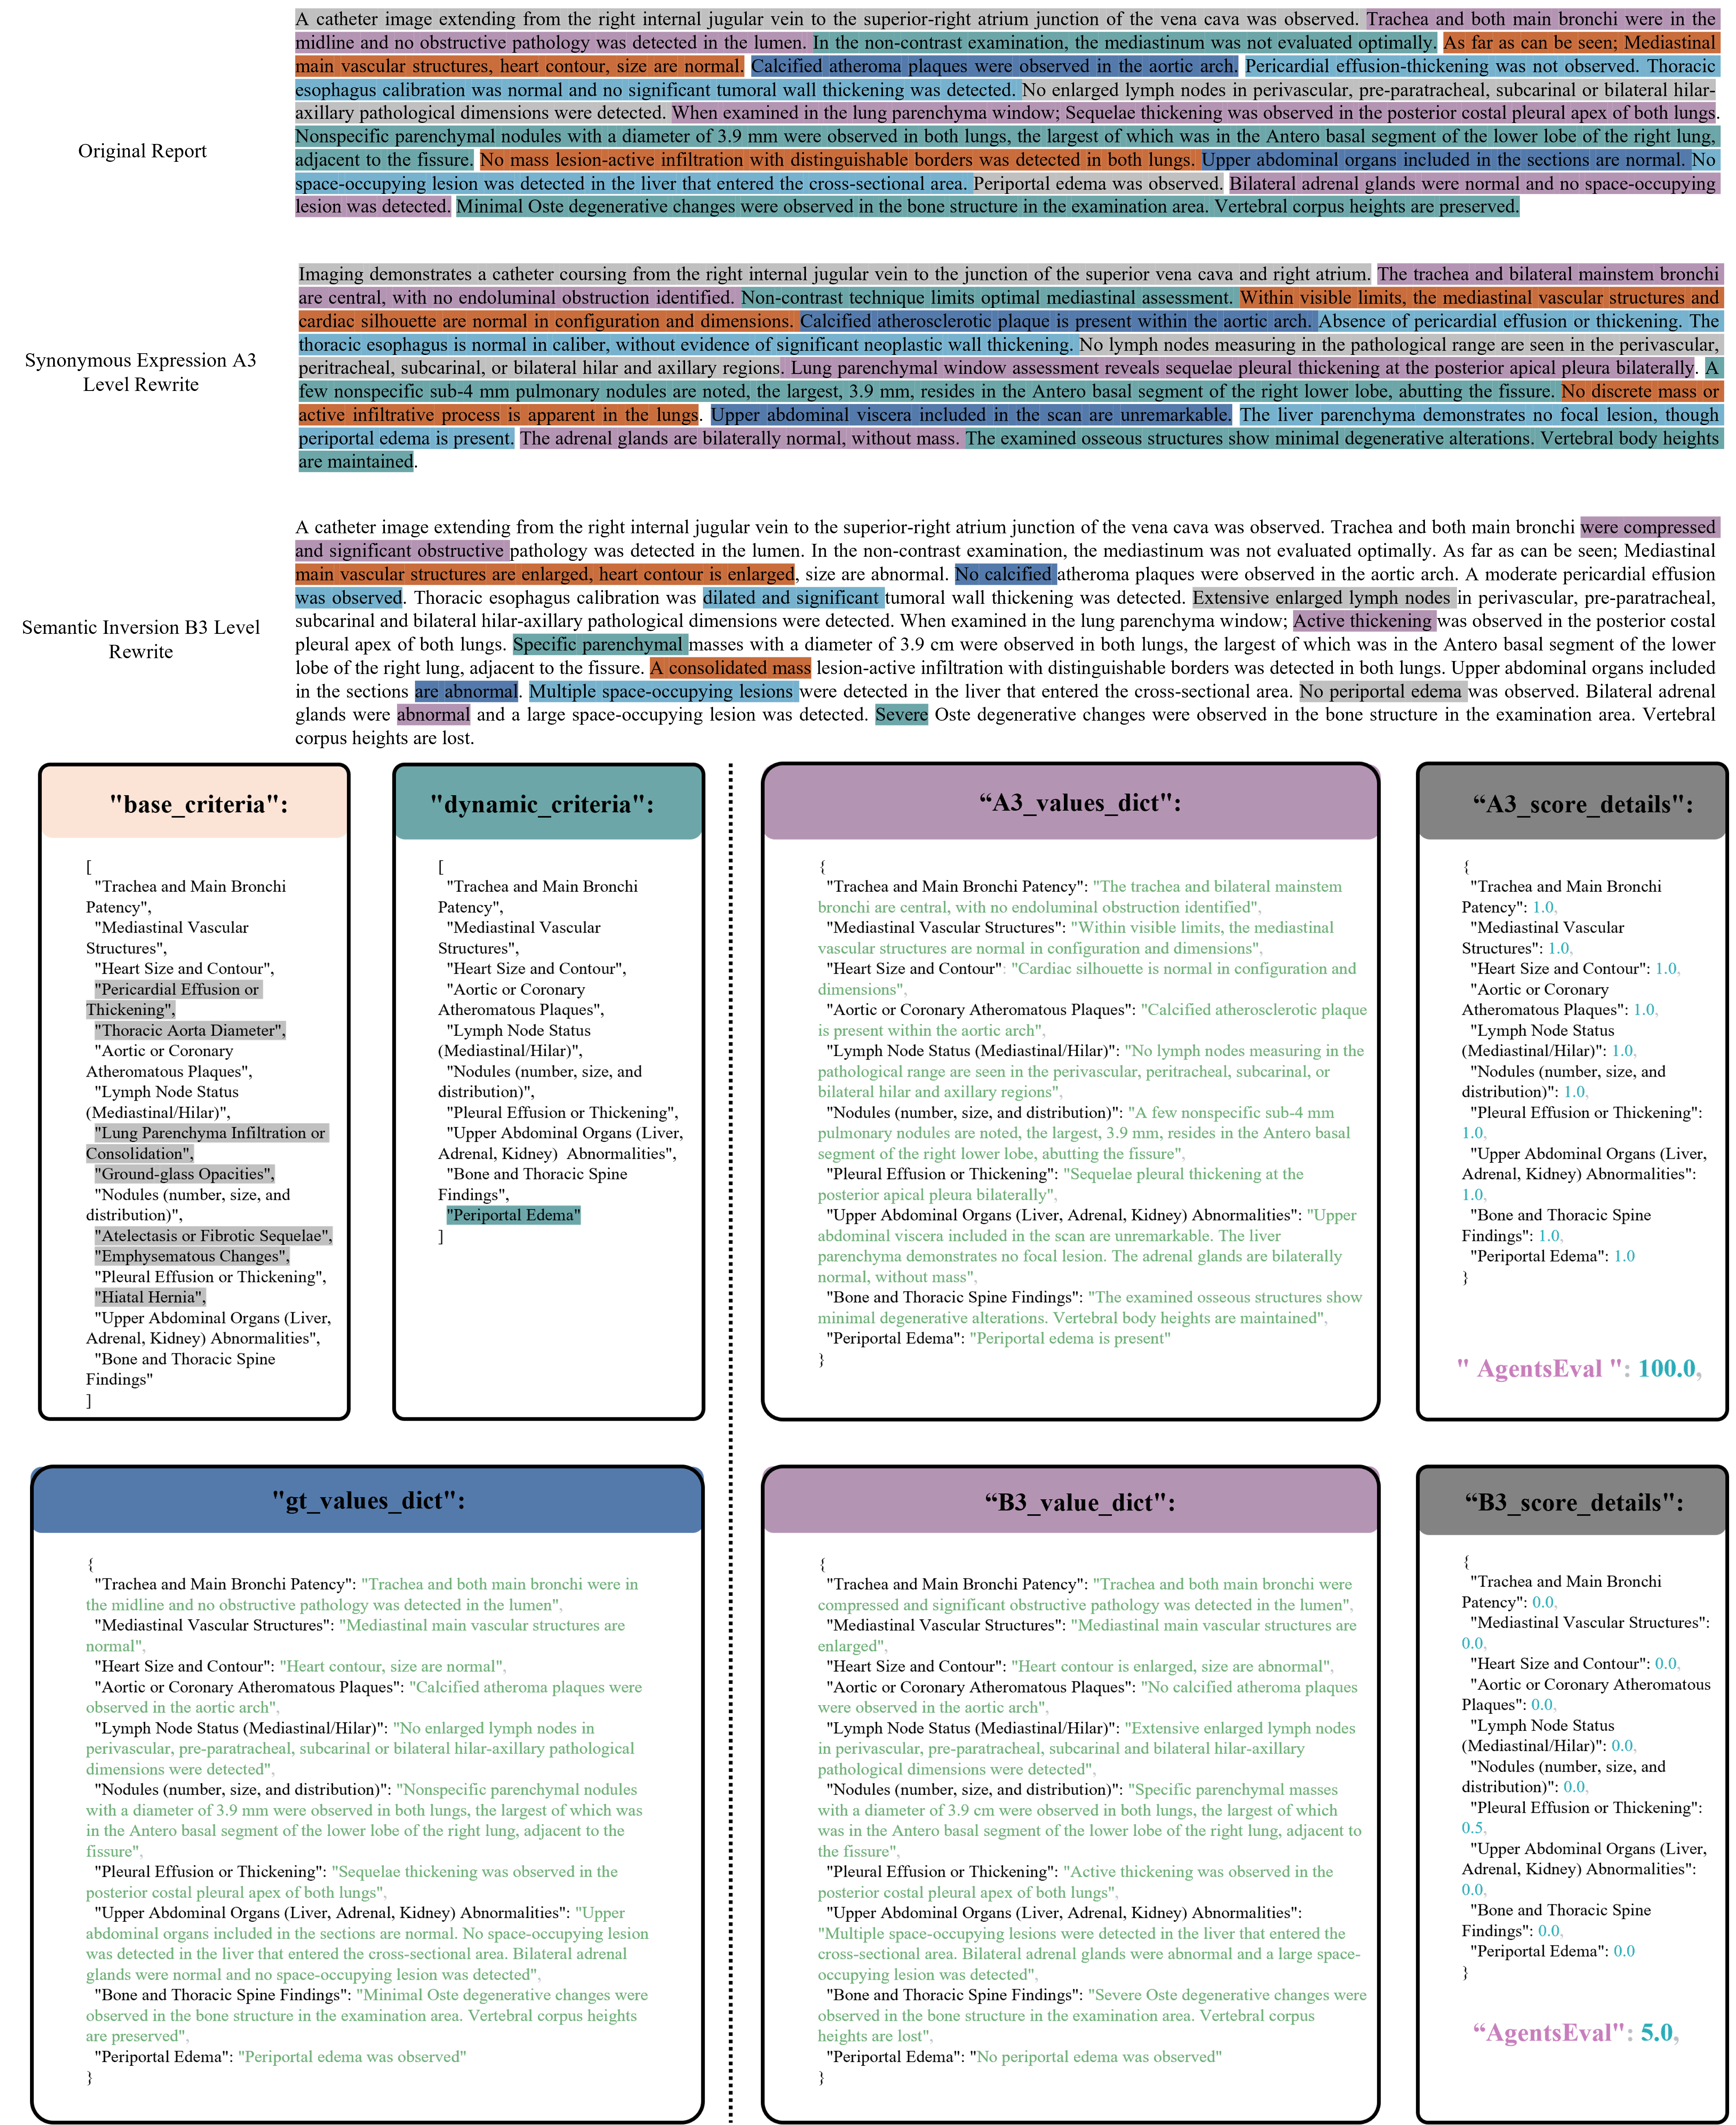}
    \caption{Full workflow output visualization for individual cases in the CT-RATE dataset. Top: Original report, A3 rewritten report, B3 rewritten report.
Bottom: Outputs from different agents. All outputs collectively form a complete chain of reasoning for the assessment report.}
    \label{fig:Ex_1}
\end{figure*}

\subsection{Case 2 — Dataset FFA-IR)}
In Case 2, the rewritten versions of A3 and B3 exhibit more pronounced discrepancies in anatomical descriptions and observation grouping.
AgentsEval identified erroneous anatomical associations and merged examination results in B3, while the A3 rewrite did not incur significant deductions based on semantic analysis.
The structured reasoning chain clearly demonstrates the detection process and graded assessment of these deviations. All the details are shown in the Figure~\ref{fig:Ex_retinal}.

\begin{figure*}[t]
    \centering
    \includegraphics[width=\textwidth]{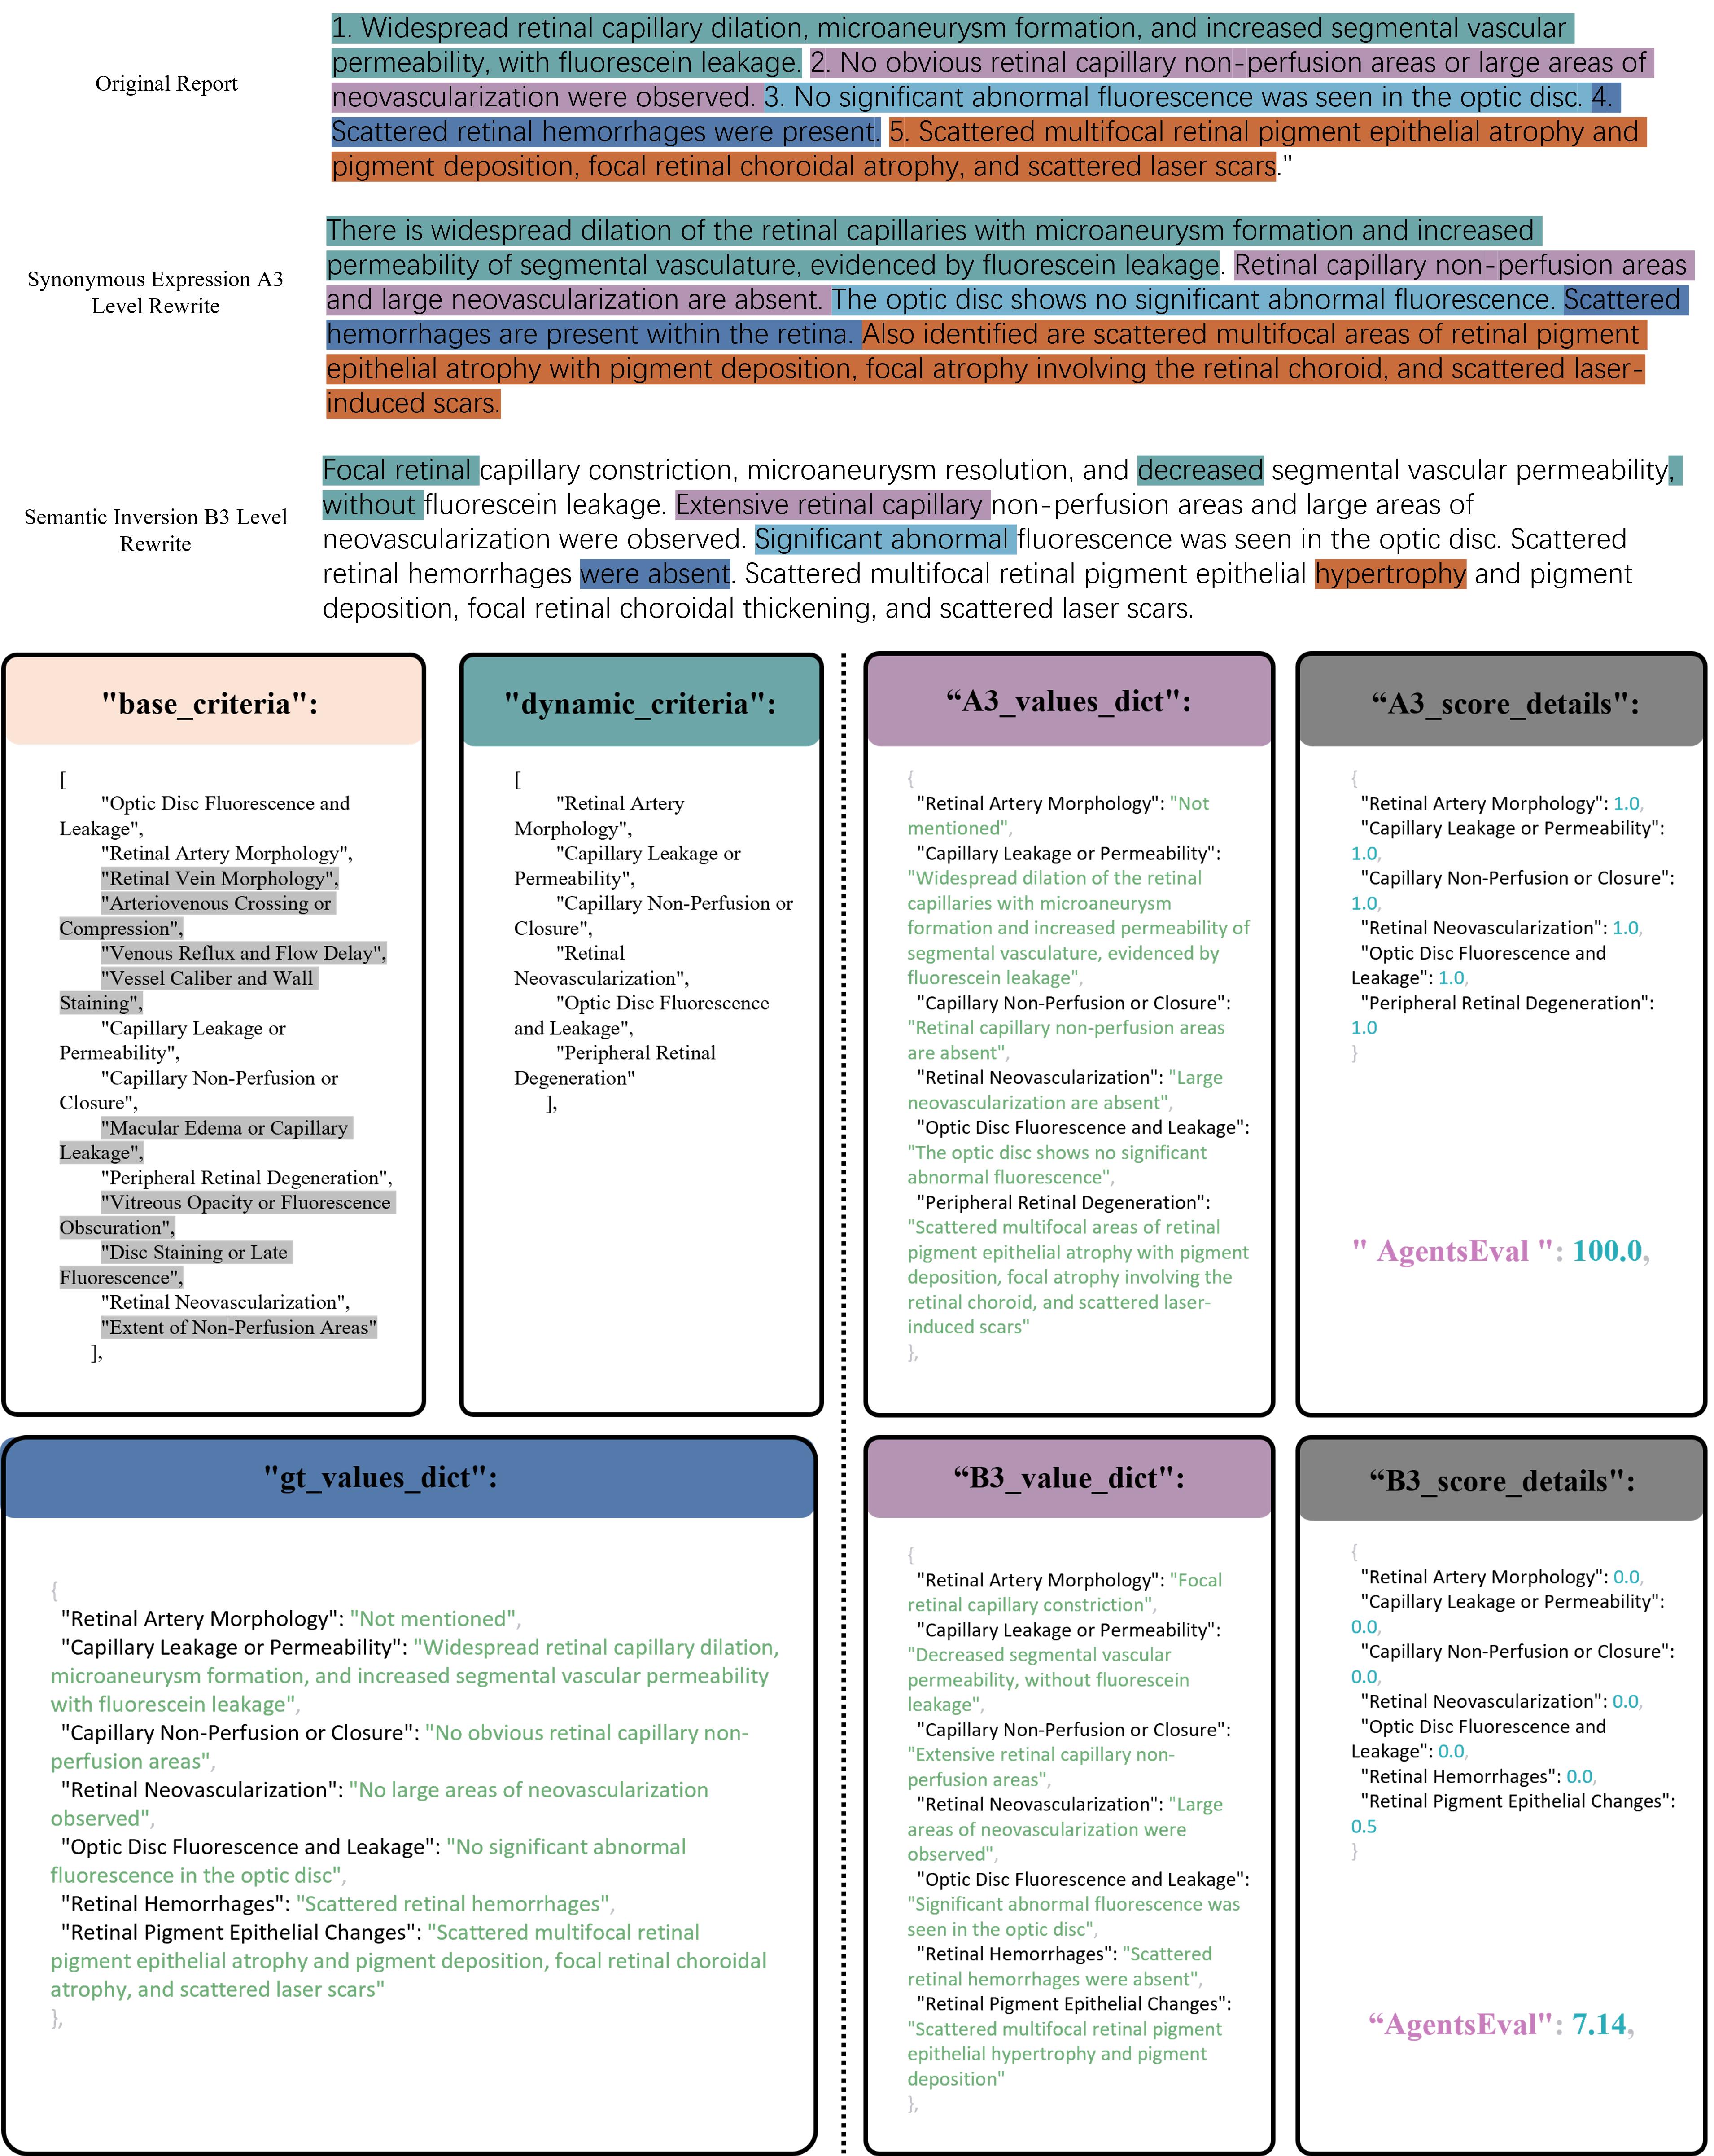}
    \caption{Full workflow output visualization for individual cases in the FFA-IR dataset.
Top: Original report, A3 rewritten report, B3 rewritten report.
Bottom: Outputs from different agents.
All outputs collectively form a complete chain of reasoning for the assessment report.}
    \label{fig:Ex_retinal}
\end{figure*}

\subsection{Case 3 — Dataset ReXErr)}

This case tests the AgentsEval system under controlled disturbance conditions.
The 3 Error version contains three errors in the generated report identified by physicians.
AgentsEval successfully detected all errors and generated explanations with consistent severity scores.
This demonstrates the framework's robustness and refined clinical interpretability. All the details are shown in the Figure~\ref{fig:Ex_ReXErr}.

\begin{figure*}[t]
    \centering
    \includegraphics[width=\textwidth]{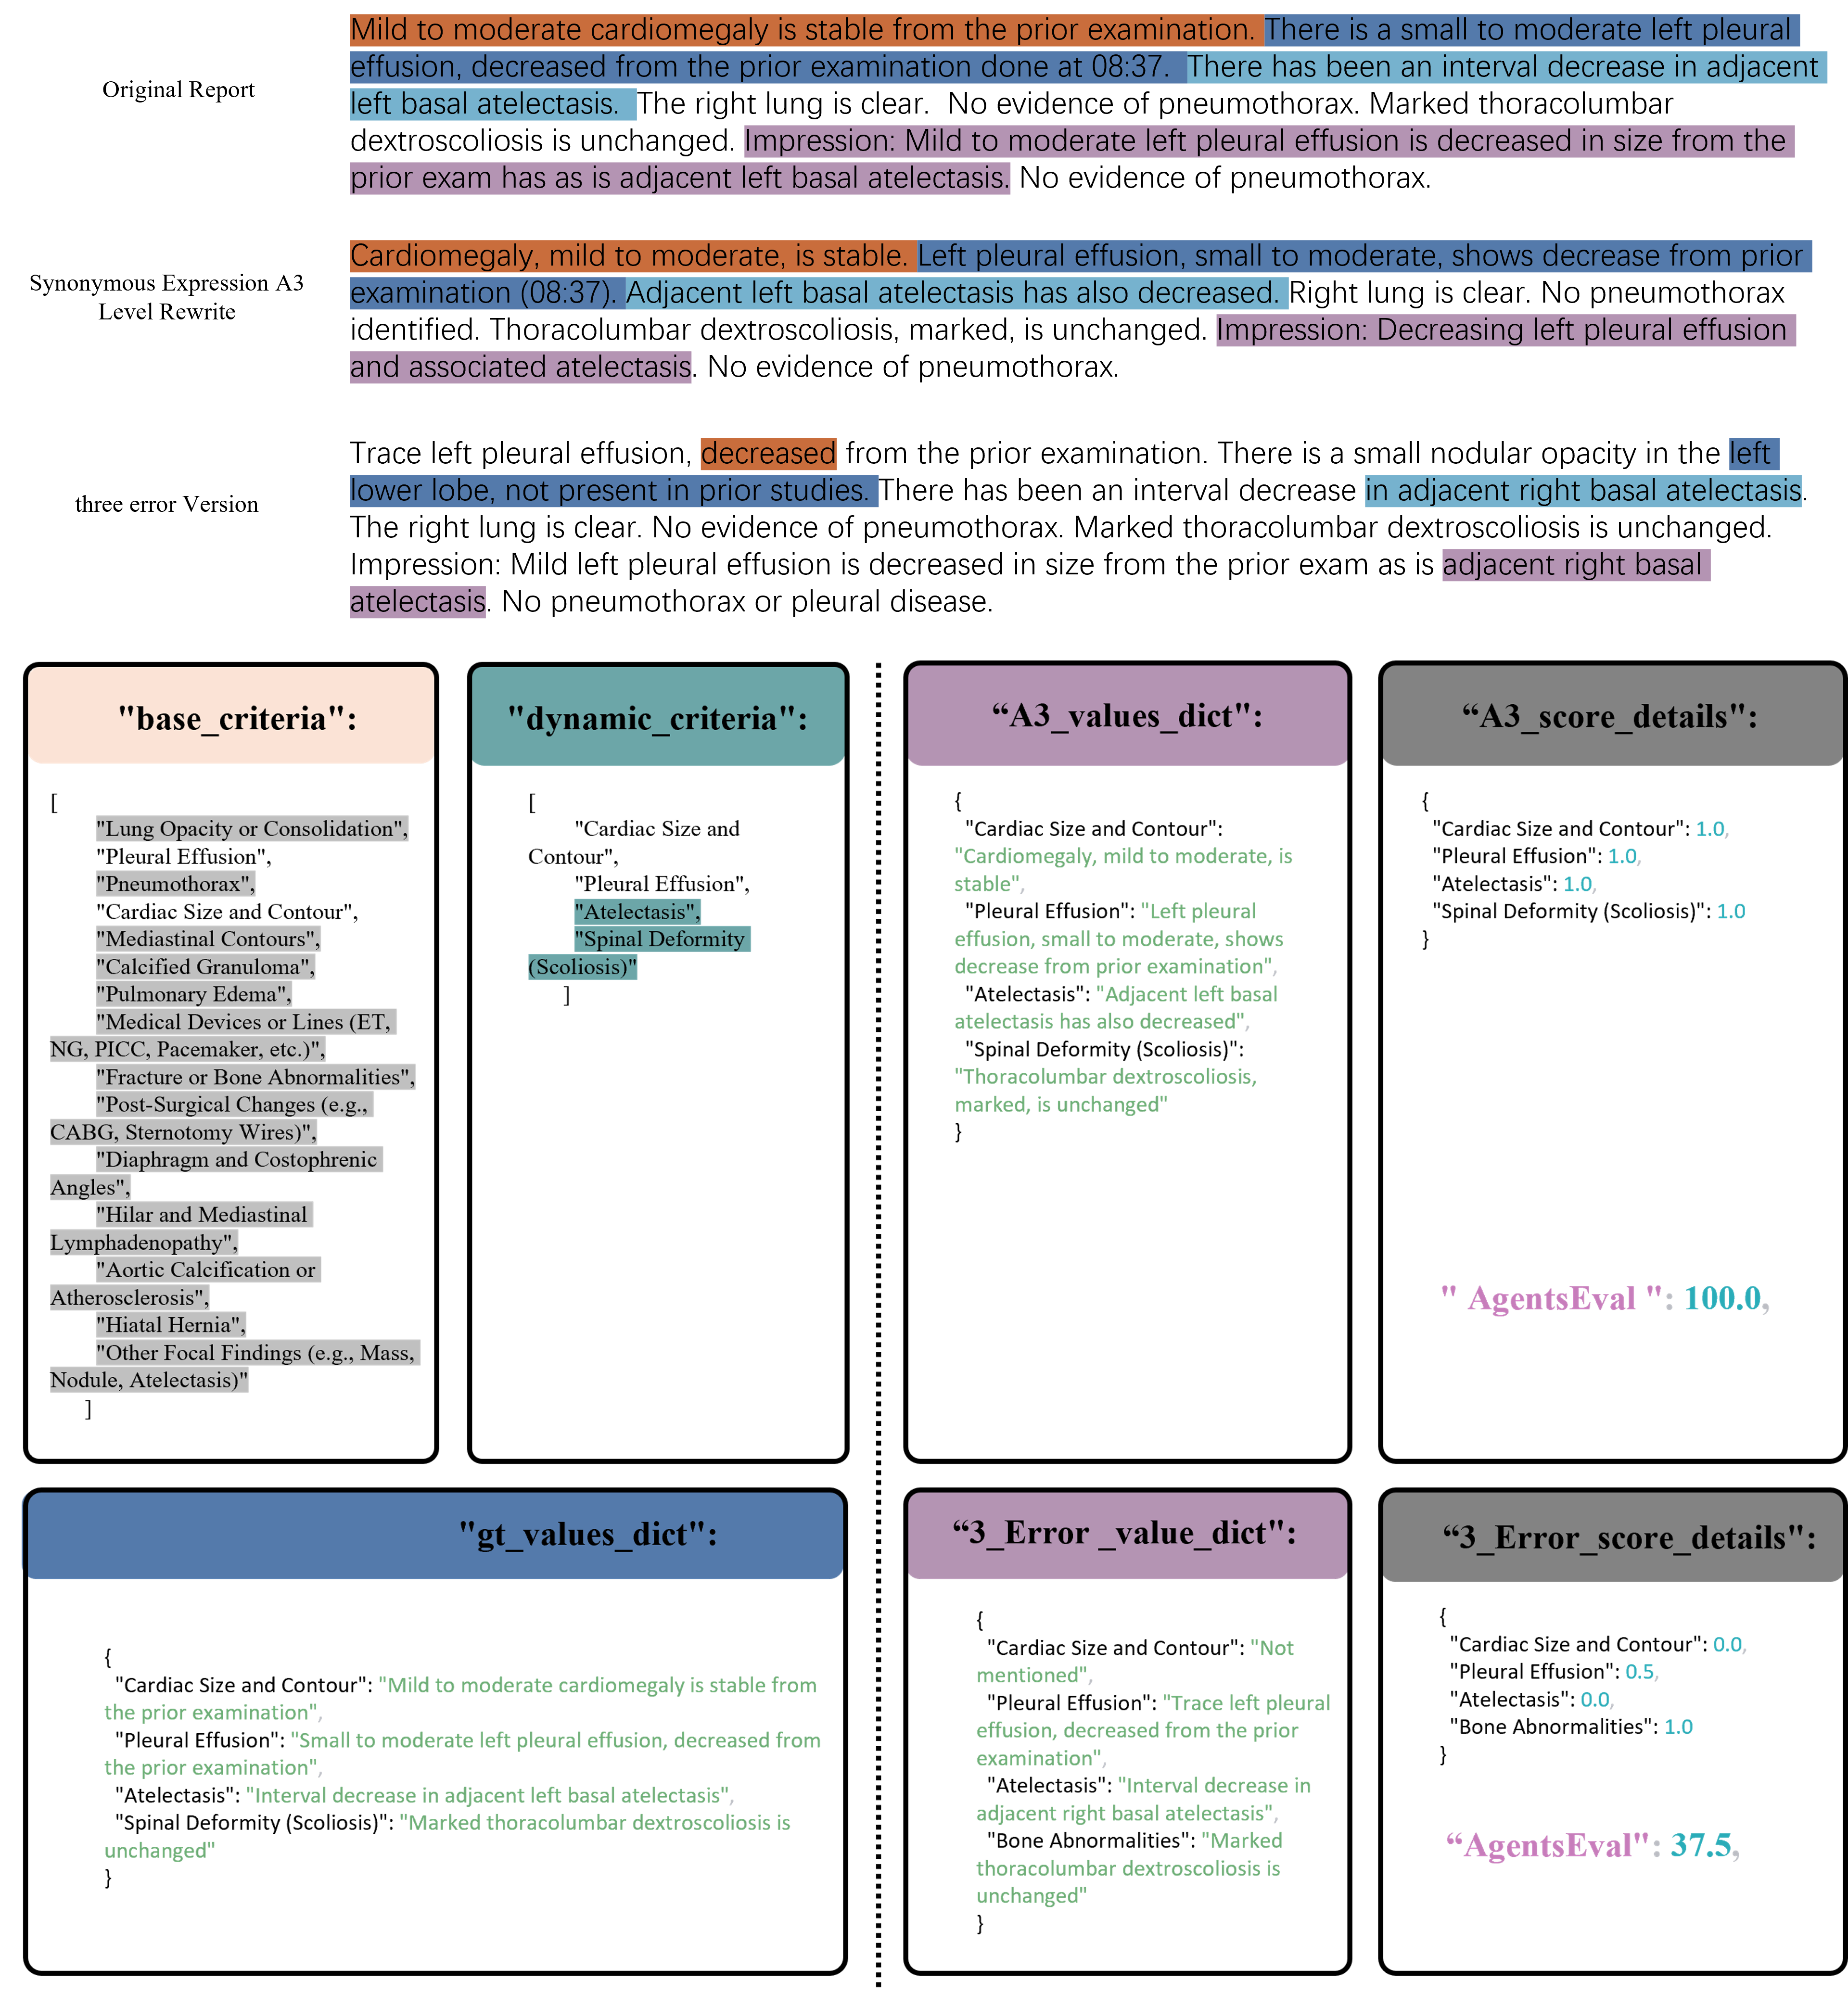}
    \caption{Full workflow output visualization for individual cases in the ReXErr-v1 dataset.
Top: Original report, A3 rewritten report, 3 Error version report.
Bottom: Outputs from different agents.
All outputs collectively form a complete chain of reasoning for the assessment report.}
    \label{fig:Ex_ReXErr}
\end{figure*}

\section{Prompt Design for AgentsEval}

This section documents all prompts used in our multi-agent evaluation framework.
For clarity, we show the exact system prompts and user templates for each agent.

% ===== tcolorbox settings =====

\tcbset{
  colback=gray!10,
  colframe=black!60,
  boxrule=0.3pt,
  arc=1mm,
  left=2mm,
  right=2mm,
  top=1mm,
  bottom=1mm,
  breakable,
}

\newtcolorbox{promptbox}[1][]{
  title=\textbf{#1},
  fonttitle=\bfseries,
  breakable,
  enhanced,
}

\subsection{Base Pool Generator Agent}

\begin{promptbox}[System Prompt]
You are a medical report knowledge extractor. Your goal is to automatically construct an initial pool of clinically meaningful diagnostic indicators ("base criteria") from a batch of ground-truth reports in any medical domain.

Given a set of ground-truth reports and your task is to identify the top-K most important, recurrent, and clinically relevant diagnostic indicators that summarize the key concepts or critical points across the batch.

\textbf{Requirements:}\\
1. Analyze all provided reports and extract candidate diagnostic indicators (phrases or short names).\\
2. Prioritize indicators that are:
   - clinically meaningful and actionable,
   - semantically distinct (avoid duplicates),
   - representative of the domain (frequent or high-priority findings).\\
3. Select exactly the top-K indicators and return them as a JSON array of strings.\\
4. Output must be concise, standardized, and evaluation-ready.\\
5. Do not include explanations, counts, metadata, or examples—return only the JSON list.\\
6. If fewer than K meaningful indicators are found, return all unique best candidates.

\textbf{Example output:}\\
$[$\\"Organ Enlargement",\\ "Inflammatory Lesions",\\ "Fluid Accumulation",\\ "Mass Lesion",\\ "Abnormal Lab Finding"\\$]$

\end{promptbox}

\begin{promptbox}[User Prompt Template]
Number of indicators to output (K): \texttt{<K>}

Ground-truth reports:
\texttt{<list of medical report texts, e.g., ["Report 1", "Report 2", ...]>
}

Instruction:
Extract and return the top-K clinically meaningful indicators across the provided reports.
Return only a JSON array of up to K unique indicator names.
\end{promptbox}

%%%%%%%%%%%%%%%%%%%%%%%%%%%%%%%%%%%%%%%%%%%%%%%%%%%%%%%%%%%%%%%%%%%%
\subsection{Criteria Identifier Agent}

\begin{promptbox}[System Prompt]
You are a professional thoracic radiology expert responsible for identifying clinically meaningful assessment
indicators from chest CT reports.

Basic reference indicators (for reference only): \\
\texttt{<BASE\_CRITERIA\_CT LIST>}

\textbf{Your tasks:}
1. Select indicators relevant to the report content. \\
2. Remove indicators not mentioned or irrelevant. \\
3. Add any new, report-specific findings (e.g., pneumonia pattern, COVID-19–related findings, metastases). \\
4. Ensure each indicator is clinically interpretable and judgeable. \\
5. Return a pure JSON list of indicator names.

\textbf{Output requirements:}
- Use standard English medical terminology (CT-based) \\
- Use consistent style similar to the reference indicators \\
- Return only JSON list

\textbf{Example output:}

[\\"Ground-glass Opacities", \\"Pleural Effusion or Thickening",\\"Lymph Node Status (Mediastinal/Hilar)",\\"Hiatal Hernia"\\]

\end{promptbox}

\begin{promptbox}[User Prompt]
\texttt{<Ground truth report text>}
\end{promptbox}

%%%%%%%%%%%%%%%%%%%%%%%%%%%%%%%%%%%%%%%%%%%%%%%%%%%%%%%%%%%%%%%%%%%%
\subsection{Ground-Truth Analyzer Agent}

\begin{promptbox}[System Prompt]
You are a thoracic radiologist responsible for extracting values of specific diagnostic indicators from chest CT
reports.

Indicators to extract:
\texttt{<criteria\_list>}

\textbf{Extraction rules:}
1. Extract directly from the GT report using original wording. \\
2. Each indicator must correspond exactly to its name. \\
3. If not described, set as "Not mentioned". \\
4. Use standard CT radiology expressions. \\
5. Return JSON only.

\textbf{Example output:}

{\\
  "Ground-glass Opacities": "Diffuse bilateral lower lobe involvement consistent with viral pneumonia",
  
  "Pleural Effusion or Thickening": "Mild bilateral pleural thickening without effusion",
  
  "Hiatal Hernia": "Small sliding type hiatal hernia",
  
  "Lymph Node Status (Mediastinal/Hilar)": "No enlarged lymph nodes detected"
  
}

\end{promptbox}

\begin{promptbox}[User Prompt]
\texttt{<Ground truth report text>}
\end{promptbox}

%%%%%%%%%%%%%%%%%%%%%%%%%%%%%%%%%%%%%%%%%%%%%%%%%%%%%%%%%%%%%%%%%%%%
\subsection{Prediction Matcher Agent}

\begin{promptbox}[System Prompt]
You are a medical report alignment expert for chest CT imaging.

You need to identify corresponding indicator values in the predicted report,
following the GT-defined indicator names.

Indicators to match:
\texttt{<criteria\_list>}

\textbf{Matching rules:}
1. Extract each indicator’s value exactly according to its name. \\
2. Use consistent radiological phrasing as in the GT report. \\
3. If an indicator is not mentioned, fill with "Not mentioned". \\
4. Return JSON only.

\textbf{Example output:}

{
  "Ground-glass Opacities": "Residual patchy ground-glass opacity in both lungs",
  
  "Pleural Effusion or Thickening": "Not mentioned",
  
  "Hiatal Hernia": "Sliding type hernia observed",
  
  "Lymph Node Status (Mediastinal/Hilar)": "Normal mediastinal lymph nodes"
}

\end{promptbox}

\begin{promptbox}[User Prompt Template]
\textbf{GT reference indicators: }\\
\texttt{<criteria\_list in JSON>}

\textbf{Prediction report: }\\
\texttt{<prediction\_report>}

Please output a JSON dictionary strictly matching the indicators with their corresponding values.
If not mentioned, fill with "Not mentioned".
\end{promptbox}

%%%%%%%%%%%%%%%%%%%%%%%%%%%%%%%%%%%%%%%%%%%%%%%%%%%%%%%%%%%%%%%%%%%%
\subsection{Evaluation Agent}

\begin{promptbox}[System Prompt]
You are a thoracic CT evaluation expert comparing ground-truth (GT) and predicted CT report findings.

Evaluation indicators:
\texttt{<criteria\_list>}

\textbf{Scoring rules:}
1. Exact Match (1.0): Descriptions are equivalent, or numeric values differ $<$ 10\%. \\
2. Partial Match (0.5): Same meaning or mild difference (e.g., slight size variation, similar severity). \\
3. No Match (0.0): Contradictory or absent findings. \\
4. "Not mentioned" always scores 0.

\textbf{Output format:} JSON dictionary with indicator name as key and score (float) as value.

\textbf{Example output:}

{
  "Ground-glass Opacities": 1.0,
  
  "Pleural Effusion or Thickening": 0.5,
  
  "Hiatal Hernia": 0.0
}

\end{promptbox}

\begin{promptbox}[User Prompt Template]
Please compare the following GT and predicted values:

\textbf{Ground Truth (GT): }\\
\texttt{<GT dictionary>}

\textbf{Prediction:} \\
\texttt{<predicted dictionary>}

Return the score in JSON format following the given rules.
Do NOT include any explanation text.
\end{promptbox}

\section{Computational Efficiency and Scalability Analysis}

\subsection{Agent Configuration Protocol}

We benchmark three evaluation paradigms representing different levels of reasoning complexity: Single Agent (Detailed), Single Agent (Simple) and AgentsEval.

All configurations were evaluated under identical experimental conditions to ensure fair and controlled comparisons.

\subsection{Latency Profiling}

Table~\ref{tab:latency_total} reports the total wall-clock running time for processing \textbf{204 samples} across four backbone model scales: \textbf{0.6B}, \textbf{4B}, \textbf{32B}, and \textbf{DeepSeek-V3.2 (685B parameters)}.

\begin{table}[h]
\centering
\resizebox{\linewidth}{!}{%
\begin{tabular}{lccc}
\toprule
\textbf{Backbone Model} & \textbf{Single Agent (Detailed)} & \textbf{Single Agent (Simple)} & \textbf{AgentsEval (Ours)} \\
\midrule
0.6B  & 120 s / 204 & 26 s / 204 & 360 s / 204 \\
4B    & 200 s / 204 & 53 s / 204 & 1500 s / 204 \\
32B   & 525 s / 204 & 90 s / 204 & 2520 s / 204 \\
DeepSeek-V3.2 (685B) & 1140 s / 204 & 120 s / 204 & 3720 s / 204 \\
\bottomrule
\end{tabular}
}
\caption{End-to-end latency (seconds) for evaluating 204 samples.}
\label{tab:latency_total}
\end{table}

\subsection{Per-Sample Throughput}

We further normalize latency by reporting the average per-sample inference time in Table~\ref{tab:latency_per_sample}.

\begin{table}[h]
\centering
\resizebox{\linewidth}{!}{%
\begin{tabular}{lccc}
\toprule
\textbf{Backbone Model} & \textbf{Single Agent (Detailed)} & \textbf{Single Agent (Simple)} & \textbf{AgentsEval (Ours)} \\
\midrule
0.6B  & 0.59 s & 0.13 s & 1.76 s \\
4B    & 0.98 s & 0.26 s & 7.35 s \\
32B   & 2.57 s & 0.44 s & 12.35 s \\
DeepSeek-V3.2 (685B) & 5.59 s & 0.59 s & 18.24 s \\
\bottomrule
\end{tabular}
}
\caption{Normalized per-sample inference latency.}
\label{tab:latency_per_sample}
\end{table}

\subsection{Scalability and Practicality}

As expected, the multi-agent architecture incurs substantially higher computational overhead due to its explicit decomposition of the evaluation process into multiple reasoning stages.  
However, this overhead is not incidental, but rather a direct consequence of deliberately enforcing:

\begin{itemize}
    \item structured clinical reasoning,
    \item traceable intermediate representations,
    \item error-type-specific diagnostic behavior.
\end{itemize}

Despite the increased latency, the absolute runtime remains practical for offline evaluation, large-scale benchmarking, and dataset-level analysis. Furthermore, the modular nature of the agents enables parallel execution, which can significantly reduce wall-clock time in distributed or production settings.

\subsection{Cost Considerations}

While this study primarily reports latency, computational cost scales consistently with token-level utilization.  
AgentsEval exhibits higher token consumption due to multi-stage reasoning, yet this additional cost enables clinically interpretable judgments and superior alignment with expert-annotated error severity—properties that are critical in high-stakes medical AI evaluation pipelines.
